# Supplementary material for: Surgeons Awareness, Expectations, and Involvement with Artificial Intelligence: a Survey Pre and Post the GPT Era
Source: arXiv:2506.08258 source file (2025-06-09)
Supplement: Supplementary file 1 [file supplementary_2.pdf]

## eMethods 2: 2024 Survey Questions

| Section      | Survey Question                                                                            |
|--------------|--------------------------------------------------------------------------------------------|
| Demographic  | Country of work *                                                                          |
|              | Gender *                                                                                   |
|              | Age *                                                                                      |
|              | Specialty *                                                                                |
|              | Main hospital setting *                                                                    |
|              | Clinical experience *                                                                      |
|              | Highest academic qualification *                                                           |
|              | Scientific experience *                                                                    |
|              | Years of research experience *                                                             |
|              | What's your affinity with new technologies? *                                              |
|              |                                                                                            |
| AI awareness | Are you familiar with the following AI terms? *                                            |
|              | Have you studied AI? *                                                                     |
|              | Have you had experience in computer programming? *                                         |
|              | Do you understand scientific articles on AI? *                                             |
|              | Are you aware of any course on AI & medicine? *                                            |
|              | If yes, which ones have you heard about?                                                   |
|              | Have you attended any course on AI & medicine? *                                           |
|              | If yes, which ones have you attended?                                                      |
|              | Would you attend a course on AI & medicine? *                                              |
|              | If yes, which of the following modalities would you prefer?                                |
|              | ChatGPT is the most common generative AI model available for public use. Have you used it? |
|              | If yes, have you ever used any AI other than ChatGPT?                                      |
|              |                                                                                            |
| Expectations | Do you think AI will be integrated into daily surgical practices? *                        |
|              | In how many years do you expect AI to be integrated into surgical practice? *              |
|              | Which segment of care will be most affected by AI within the next 10 years?                |
|              | What do you think will be the role of AI in surgery within the next 10 years?              |
|              | What do you think are the most important uses of surgical AI?                              |
|              | What do you think are the main barriers to implementing AI in surgical practices?          |
|              | Do you think AI will impact your job as a surgeon? *                                       |
|              | Which would you prefer to use: AI tool 1 (more accurate) or AI tool 2 (more explainable)?  |
|              | Can you think of any risks related to the use of AI in surgery? *                          |
|              | If yes, please tell us more about the foreseen risk:                                       |
|              |                                                                                            |
| Involvement  | Are you involved in Surgical AI research or development? *                                 |
|              | Do you or your institution collect surgical data? *                                        |
|              | Have you ever annotated/labeled surgical data *                                            |
|              | Have you ever collaborated with engineers in a surgical AI project? *                      |

## eMethods 2: 2024 Survey Questions

|                               |                                                                                                                                                                     |
|-------------------------------|---------------------------------------------------------------------------------------------------------------------------------------------------------------------|
|                               | Who do you think should take the lead in researching surgical AI? *                                                                                                 |
|                               | Are you involved with the Surgical Data Science (SDS) research community? *                                                                                         |
|                               | Are you willing to use surgical AI tools in your practice? *                                                                                                        |
|                               | Are you recording your cases on a daily basis? *                                                                                                                    |
|                               | If not, what are the hurdles for you not recording?                                                                                                                 |
|                               | If not, what could incentive surgeons to systematically record cases?                                                                                               |
| <b>Ethical Considerations</b> | How concerned are you about the potential for ethical issues arising from the use of AI in surgery?                                                                 |
|                               | How important is it to address ethical considerations when implementing AI in surgical practices?                                                                   |
|                               | What do you believe are the main ethical concerns associated with AI in surgery? (Select all that apply)                                                            |
|                               | How important do you think it is for AI systems used in surgery to be explainable?                                                                                  |
|                               | What measures do you think can enhance the explainability of AI systems in surgery? (Select all that apply)                                                         |
|                               | What measures do you think are necessary to ensure the responsible use of AI in surgery? (Select all that apply)                                                    |
|                               | What steps do you think can be taken to mitigate algorithmic bias in surgical AI? (Select all that apply)                                                           |
|                               | How concerned are you about the possibility of errors in treatment decisions due to AI recommendations?                                                             |
|                               | What measures do you think can be taken to minimize errors in treatment decisions related to AI use? (Select all that apply)                                        |
|                               | How concerned are you about the potential intervention of private interests in the development and use of AI in surgery?                                            |
|                               | What steps do you think can be taken to ensure that AI development and use in surgery remain free from undue private interest intervention? (Select all that apply) |
| <b>Have your say</b>          | If you wish, let us know your opinion on surgical AI, important unmet surgical needs, procedures/problems to focus on, etc.                                         |
|                               | If you would like to receive updates on the findings from this questionnaire or be informed about future AI in surgery projects, please leave your email address    |

\* Mandatory question
