# Supplementary material for: Surgeons Awareness, Expectations, and Involvement with Artificial Intelligence: a Survey Pre and Post the GPT Era
Source: arXiv:2506.08258 source file (2025-06-09)
Supplement: Supplementary file 2 [file supplementary_3.pdf]

**eTable 1. Predictors of surgeons' perceptions and involvement with AI across key domains (2021 and 2024)**

|                                                                                                                  |                                                                                                   | Independent Vars - Predictors                                       | Coefficient (c) | p-value |
|------------------------------------------------------------------------------------------------------------------|---------------------------------------------------------------------------------------------------|---------------------------------------------------------------------|-----------------|---------|
| <b>A I<br/>I<br/>N<br/>T<br/>E<br/>G<br/>R<br/>A<br/>T<br/>I<br/>O<br/>N</b>                                     | <b>Dependent Var: In how many years do you expect AI to be integrated into surgical practice?</b> |                                                                     |                 |         |
|                                                                                                                  | <b>2021</b>                                                                                       | Scientific experience                                               | 0.0789          | 0.041   |
|                                                                                                                  |                                                                                                   | Have you studied AI?                                                | -0.1921         | 0.002   |
|                                                                                                                  |                                                                                                   | Would you attend a course on AI & medicine?                         | 0.1349          | 0.025   |
|                                                                                                                  |                                                                                                   | Do you understand scientific articles on AI?                        | 0.1165          | 0.042   |
|                                                                                                                  | <b>2024</b>                                                                                       | What's your affinity with new technologies?                         | 0.2568          | 0.028   |
| <b>A I<br/>F<br/>A<br/>M<br/>I<br/>L<br/>I<br/>A<br/>R<br/>I<br/>T<br/>Y</b>                                     | <b>Dependent Var: Do you understand scientific articles on AI?</b>                                |                                                                     |                 |         |
|                                                                                                                  | <b>2021</b>                                                                                       | Age                                                                 | 0.0078          | 0.031   |
|                                                                                                                  |                                                                                                   | What's your affinity with new technologies?                         | 0.1025          | 0.003   |
|                                                                                                                  |                                                                                                   | Are you familiar with the following AI terms?                       | 0.1646          | < 0.001 |
|                                                                                                                  |                                                                                                   | Have you studied AI?                                                | 0.2697          | < 0.001 |
|                                                                                                                  |                                                                                                   | Have you had experience in computer programming?                    | 0.1340          | < 0.001 |
|                                                                                                                  | <b>2024</b>                                                                                       | Have you had experience in computer programming?                    | 0.2400          | 0.013   |
|                                                                                                                  |                                                                                                   | Have you ever collaborated with engineers in a surgical AI project? | 0.2509          | 0.025   |
| <b>A I<br/>R<br/>E<br/>S<br/>E<br/>A<br/>R<br/>C<br/>H<br/>I<br/>N<br/>V<br/>O<br/>L<br/>V<br/>E<br/>M<br/>E</b> | <b>Dependent Var: Are you involved in Surgical AI research or development?</b>                    |                                                                     |                 |         |
|                                                                                                                  | <b>2021</b>                                                                                       | Age                                                                 | -0.0079         | 0.049   |
|                                                                                                                  |                                                                                                   | Scientific experience                                               | 0.0956          | 0.006   |
|                                                                                                                  |                                                                                                   | Are you familiar with the following AI terms?                       | 0.1127          | 0.006   |
|                                                                                                                  |                                                                                                   | Do you understand scientific articles on AI?                        | 0.1042          | 0.046   |
|                                                                                                                  | <b>2024</b>                                                                                       | Have you studied AI?                                                | 0.3926          | 0.0246  |
|                                                                                                                  |                                                                                                   | Have you ever collaborated with engineers in a surgical AI project? | 0.4530          | < 0.001 |
|                                                                                                                  | <b>Dependent Var: Are you involved with the Surgical Data Science (SDS) research community?</b>   |                                                                     |                 |         |
|                                                                                                                  | <b>2021</b>                                                                                       | Do you understand scientific articles on AI?                        | 0.1236          | 0.020   |
|                                                                                                                  |                                                                                                   | Are you involved in Surgical AI research or development?            | 0.2205          | 0.002   |

|                                                                                                                      |                                                                                                                                                                         |                                                                             |        |       |
|----------------------------------------------------------------------------------------------------------------------|-------------------------------------------------------------------------------------------------------------------------------------------------------------------------|-----------------------------------------------------------------------------|--------|-------|
| N<br>T                                                                                                               | 2024                                                                                                                                                                    | Have you ever collaborated with engineers in a surgical AI project?         | 0.3320 | 0.022 |
|                                                                                                                      | <b>Dependent Var: Would you use a system that prioritizes accuracy or explainability? *</b><br><b>Higher values correspond to explainable, lower values to accurate</b> |                                                                             |        |       |
| A<br>C<br>C<br>V<br>S<br>E<br>X<br>P<br>A<br>I<br>I<br>M<br>P<br>L<br>E<br>M<br>E<br>N<br>T<br>A<br>T<br>I<br>O<br>N | 2021                                                                                                                                                                    | Are you familiar with the following AI terms?                               | 0.1181 | 0.044 |
|                                                                                                                      | 2024                                                                                                                                                                    | Do you understand scientific articles on AI?                                | 0.3403 | 0.031 |
|                                                                                                                      |                                                                                                                                                                         | Do you think AI will be integrated into daily surgical practices?           | 0.4911 | 0.013 |
|                                                                                                                      | <b>Dependent Var: Do you think AI will impact your job as a surgeon?</b>                                                                                                |                                                                             |        |       |
|                                                                                                                      | 2021                                                                                                                                                                    | In how many years do you expect AI to be integrated into surgical practice? | 0.0900 | 0.047 |
|                                                                                                                      |                                                                                                                                                                         | Are you willing to use surgical AI tools in your practice?                  | 0.2070 | 0.003 |
|                                                                                                                      | <b>Dependent Var: Are you willing to use surgical AI tools in your practice?</b>                                                                                        |                                                                             |        |       |
|                                                                                                                      | 2021                                                                                                                                                                    | What's your affinity with new technologies?                                 | 0.0830 | 0.002 |
|                                                                                                                      |                                                                                                                                                                         | Have you studied AI?                                                        | 0.0932 | 0.017 |
|                                                                                                                      |                                                                                                                                                                         | Do you think AI will be integrated into daily surgical practices?           | 0.0916 | 0.033 |
|                                                                                                                      |                                                                                                                                                                         |                                                                             |        |       |
