# Supplementary material for: Surgeons Awareness, Expectations, and Involvement with Artificial Intelligence: a Survey Pre and Post the GPT Era
Source: arXiv:2506.08258 source file (2025-06-09)
Supplement: Supplementary file 3 [file supplementary_4.pdf]

**eTable 2. Distribution of answers about ethical considerations, distributed only in the 2024 edition of the survey.**

| Answer                                                                                                             | Count        |
|--------------------------------------------------------------------------------------------------------------------|--------------|
| <b>How concerned are you about the potential for ethical issues arising from the use of AI in surgery?</b>         |              |
| Very concerned                                                                                                     | 23 (15.54 %) |
| Concerned                                                                                                          | 45 (30.41 %) |
| Slightly concerned                                                                                                 | 58 (39.19 %) |
| Not concerned                                                                                                      | 16 (10.81 %) |
| Not reported                                                                                                       | 6 (4.05 %)   |
| <b>How important is it to address ethical considerations when implementing AI in surgical practices?</b>           |              |
| Very important                                                                                                     | 65 (43.92 %) |
| Important                                                                                                          | 58 (39.19 %) |
| Slightly important                                                                                                 | 16 (10.81 %) |
| Not important                                                                                                      | 2 (1.35 %)   |
| Not reported                                                                                                       | 7 (4.73 %)   |
| <b>What do you believe are the main ethical concerns associated with AI in surgery? (Multiple answers allowed)</b> |              |
| Accountability and transparency of AI decisions                                                                    | 89 (25.36 %) |
| Patient privacy and data security                                                                                  | 75 (21.37 %) |
| Algorithmic bias and fairness                                                                                      | 67 (19.09 %) |
| Informed consent for AI-assisted procedures                                                                        | 64 (18.23 %) |
| Impact on surgeon-patient relationship                                                                             | 56 (15.95 %) |
| <b>How important do you think it is for AI systems used in surgery to be explainable?</b>                          |              |
| Very important                                                                                                     | 73 (49.32 %) |
| Important                                                                                                          | 48 (32.43 %) |
| Slightly important                                                                                                 | 19 (12.84 %) |
| Not important                                                                                                      | 2 (1.35 %)   |
| Not reported                                                                                                       | 6 (4.05 %)   |

| Answer                                                                                                                     | Count         |
|----------------------------------------------------------------------------------------------------------------------------|---------------|
| <b>What measures do you think can enhance the explainability of AI systems in surgery? (Multiple answers allowed)</b>      |               |
| Collaboration between AI developers and surgeons                                                                           | 109 (26.20 %) |
| Regular training sessions and workshops                                                                                    | 91 (21.88 %)  |
| Visual aids and explanatory tools within AI interfaces                                                                     | 84 (20.19 %)  |
| Transparent reporting of AI system performance and updates                                                                 | 73 (17.55 %)  |
| Clear documentation and user manuals                                                                                       | 58 (13.94 %)  |
| Not reported                                                                                                               | 1 (0.24 %)    |
| <b>What measures do you think are necessary to ensure the responsible use of AI in surgery? (Multiple answers allowed)</b> |               |
| Comprehensive training programs for surgeons                                                                               | 115 (23.76 %) |
| Transparent reporting of adverse events                                                                                    | 100 (20.66 %) |
| Regular audits and monitoring of AI systems                                                                                | 95 (19.63 %)  |
| Implementing ethical guidelines and standards                                                                              | 93 (19.21 %)  |
| Ensuring data integrity and privacy                                                                                        | 79 (16.32 %)  |
| Closer integration of CS (computer science) specialists in OR (operating room)/surgical practice                           | 1 (0.21 %)    |
| Dynamic rectification of errors                                                                                            | 1 (0.21 %)    |
| <b>What steps do you think can be taken to mitigate algorithmic bias in surgical AI? (Multiple answers allowed)</b>        |               |
| Inclusion of multidisciplinary teams in ai development                                                                     | 88 (22.68 %)  |
| Continuous monitoring and improvement                                                                                      | 85 (21.91 %)  |
| Regular bias audits and testing                                                                                            | 77 (19.85 %)  |
| Transparent algorithm development processes                                                                                | 73 (18.81 %)  |
| Diverse and representative training data                                                                                   | 65 (16.75 %)  |
| <b>How concerned are you about the possibility of errors in treatment decisions due to AI recommendations?</b>             |               |
| Concerned                                                                                                                  | 67 (45.27 %)  |
| Not concerned                                                                                                              | 3 (2.03 %)    |
| Slightly concerned                                                                                                         | 31 (20.95 %)  |

| Answer                                                                                                                                                                        | Count         |
|-------------------------------------------------------------------------------------------------------------------------------------------------------------------------------|---------------|
| Not reported                                                                                                                                                                  | 8 (5.41 %)    |
| <b>What measures do you think can be taken to minimize errors in treatment decisions related to AI use? (Multiple answers allowed)</b>                                        |               |
| Comprehensive training for surgeons on AI limitations and strengths                                                                                                           | 117 (29.70 %) |
| Continuous monitoring and validation of AI systems                                                                                                                            | 100 (25.38 %) |
| Regular updates and improvements to AI algorithms                                                                                                                             | 91 (23.10 %)  |
| Involvement of multidisciplinary teams in decision-making                                                                                                                     | 84 (21.32 %)  |
| I am not a specialist of AI to answer that                                                                                                                                    | 1 (0.25 %)    |
| Pre and post operative outcome records using AI                                                                                                                               | 1 (0.25 %)    |
| <b>How concerned are you about the potential intervention of private interests in the development and use of AI in surgery?</b>                                               |               |
| Very concerned                                                                                                                                                                | 37 (25.00 %)  |
| Concerned                                                                                                                                                                     | 54 (36.49 %)  |
| Slightly concerned                                                                                                                                                            | 38 (25.68 %)  |
| Not concerned                                                                                                                                                                 | 11 (7.43 %)   |
| Not reported                                                                                                                                                                  | 8 (5.41 %)    |
| <b>What steps do you think can be taken to ensure that AI development and use in surgery remain free from undue private interest intervention? (Multiple answers allowed)</b> |               |
| Establishing clear ethical guidelines and standards                                                                                                                           | 100 (27.70 %) |
| Transparency in AI development and funding sources                                                                                                                            | 99 (27.42 %)  |
| Independent audits and reviews of AI systems                                                                                                                                  | 88 (24.38 %)  |
| Involvement of regulatory bodies in oversight                                                                                                                                 | 72 (19.94 %)  |
| Like any other technology in the OR. No difference                                                                                                                            | 1 (0.28 %)    |
| I feel it is difficult to avoid private interest. but we can limit. funding can be an issue if we want complete free private intervention                                     | 1 (0.28 %)    |
